# Supplementary material for: Superstabilizing Control of Discrete-Time ARX Models under Error in Variables
Source: arXiv:2210.14893 source file (2023-07-10)
Supplement: Supplementary file 1 [file appendix.tex]

\appendix
\section{Optional Appendix}    % Each appendix must have a short title.
\section{More Appendices}              % Sections and subsections are supported  
